# Supplementary material for: Non-parametric estimation of transition intensities in interval censored Markov multi-state models without loops
Source: arXiv:2409.07176 source file (2025-07-15)
Supplement: Supplementary file 1 [file SupplementaryMaterial.tex]

\documentclass{article}

\usepackage{PRIMEarxiv}

\usepackage{moreverb,url}
\usepackage{bm}
\usepackage{graphicx}
\usepackage{soul}
\usepackage{caption, subcaption}
\usepackage{amsmath}
\usepackage{dsfont}
\usepackage{mathtools}
\usepackage{amssymb}
\usepackage{prodint}
\usepackage[symbol, bottom]{footmisc}

\usepackage[utf8]{inputenc} % allow utf-8 input
\usepackage[T1]{fontenc}    % use 8-bit T1 fonts
\usepackage{hyperref}       % hyperlinks
\usepackage{url}            % simple URL typesetting
\usepackage{booktabs}       % professional-quality tables
\usepackage{amsfonts}       % blackboard math symbols
\usepackage{nicefrac}       % compact symbols for 1/2, etc.
\usepackage{microtype}      % microtypography
\usepackage{lipsum}
\usepackage{fancyhdr}       % header
\usepackage{graphicx}       % graphics
\graphicspath{{figures/}}     % organize your images and other figures under media/ folder

\usepackage{tikz}
\usetikzlibrary{arrows}

\newcommand{\stkout}[1]{\ifmmode\text{\sout{\ensuremath{#1}}}\else\sout{#1}\fi}

%Header
\pagestyle{fancy}
\thispagestyle{empty}
\rhead{ \textit{ }} 

% Update your Headers here
\fancyhead[LO]{Gomon and Putter}
% \fancyhead[RE]{Firstauthor and Secondauthor} % Firstauthor et al. if more than 2 - must use \documentclass[twoside]{article}

%% Title
\title{Supplemental material to Non-parametric estimation of transition intensities in interval censored Markovian multi-state models without loops
%%%% Cite as
%%%% Update your official citation here when published 
%\thanks{\textit{\underline{Citation}}: 
%\textbf{Authors. Title. Pages.... DOI:000000/11111.}} 
}

\author{
  %Daniel Gomon \\
  %Mathematical Institute \\
  %Leiden University \\
  %Leiden, the Netherlands\\
  %% examples of more authors
  % \And
  %Hein Putter \\
  %Department of Biomedical Data Sciences \\
  %Leiden University Medical Centre \\
  %Leiden, the Netherlands\\
  %% \AND
  %% Coauthor \\
  %% Affiliation \\
  %% Address \\
  %% \texttt{email} \\
  %% \And
  %% Coauthor \\
  %% Affiliation \\
  %% Address \\
  %% \texttt{email} \\
  %% \And
  %% Coauthor \\
  %% Affiliation \\
  %% Address \\
  %% \texttt{email} \\
}

\begin{document}
\maketitle

\vspace{-7em}
\begin{center}
% authors go here:
\large{
Daniel Gomon \textsuperscript{1,}\footnote[1]{Corresponding Author, d.gomon@math.leidenuniv.nl},
Hein Putter \textsuperscript{1,2}}
\\
\bigskip
\normalsize
\textit{\textsuperscript{1} Mathematical Institute, Leiden University, Einsteinweg 55, Leiden, the Netherlands}
\\
\textit{\textsuperscript{2} Department of Biomedical Data Sciences, Leiden University Medical Centre, Einthovenweg 20, Leiden, the Netherlands}
\\
\bigskip
\end{center}

\section{Simulation Study - Figures}

This section presents the complete results concerning performance measures in the six considered scenarios.

\begin{figure}[!ht]
    \centering
    \includegraphics[width = 0.9 \textwidth]{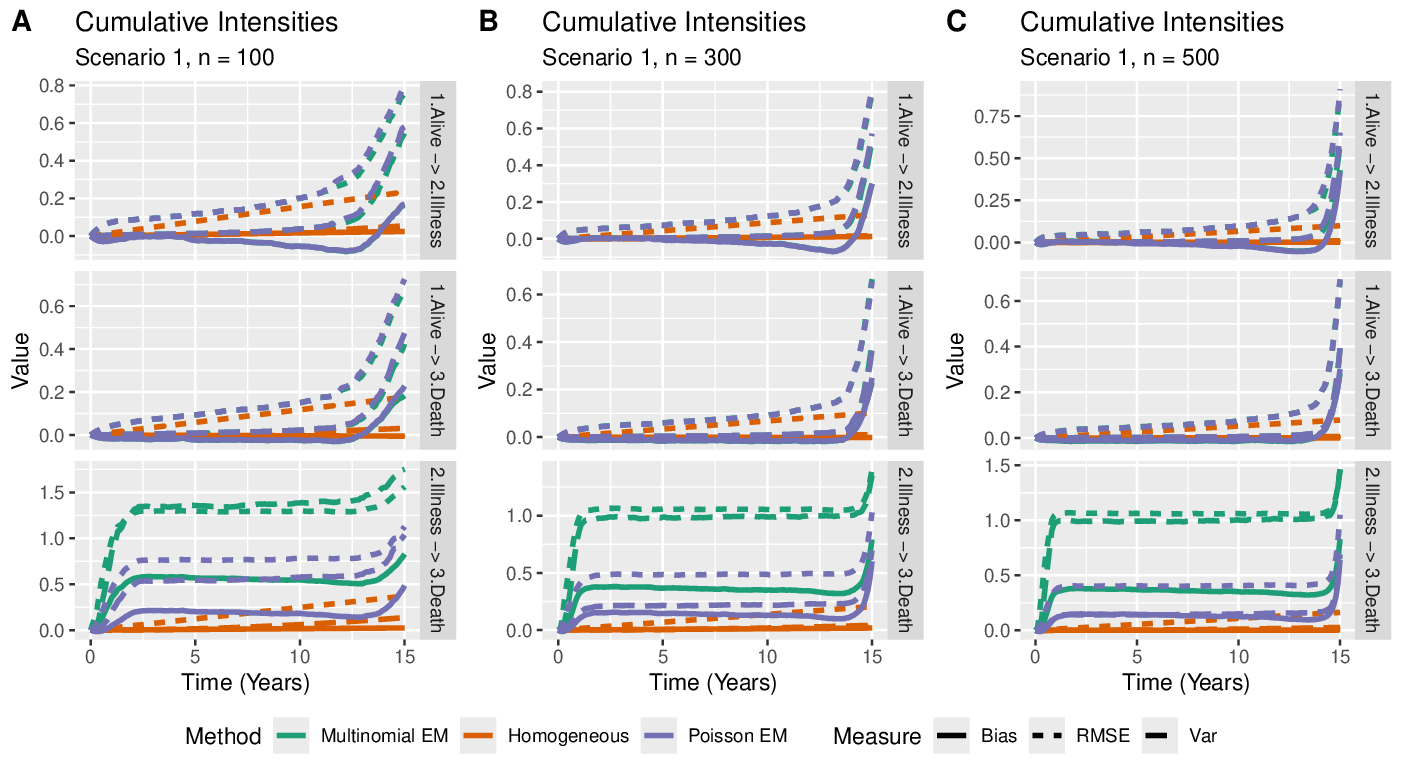}
    \caption{Bias, Variance and RMSE of cumulative intensities in scenario 1 for A) $n = 100$, B) $n = 300$, C) $n = 500$ samples in $N = 1000$ simulated data sets.}
    \label{fig:sc1int}
\end{figure}

\begin{figure}[!ht]
    \centering
    \includegraphics[width = 0.9 \textwidth]{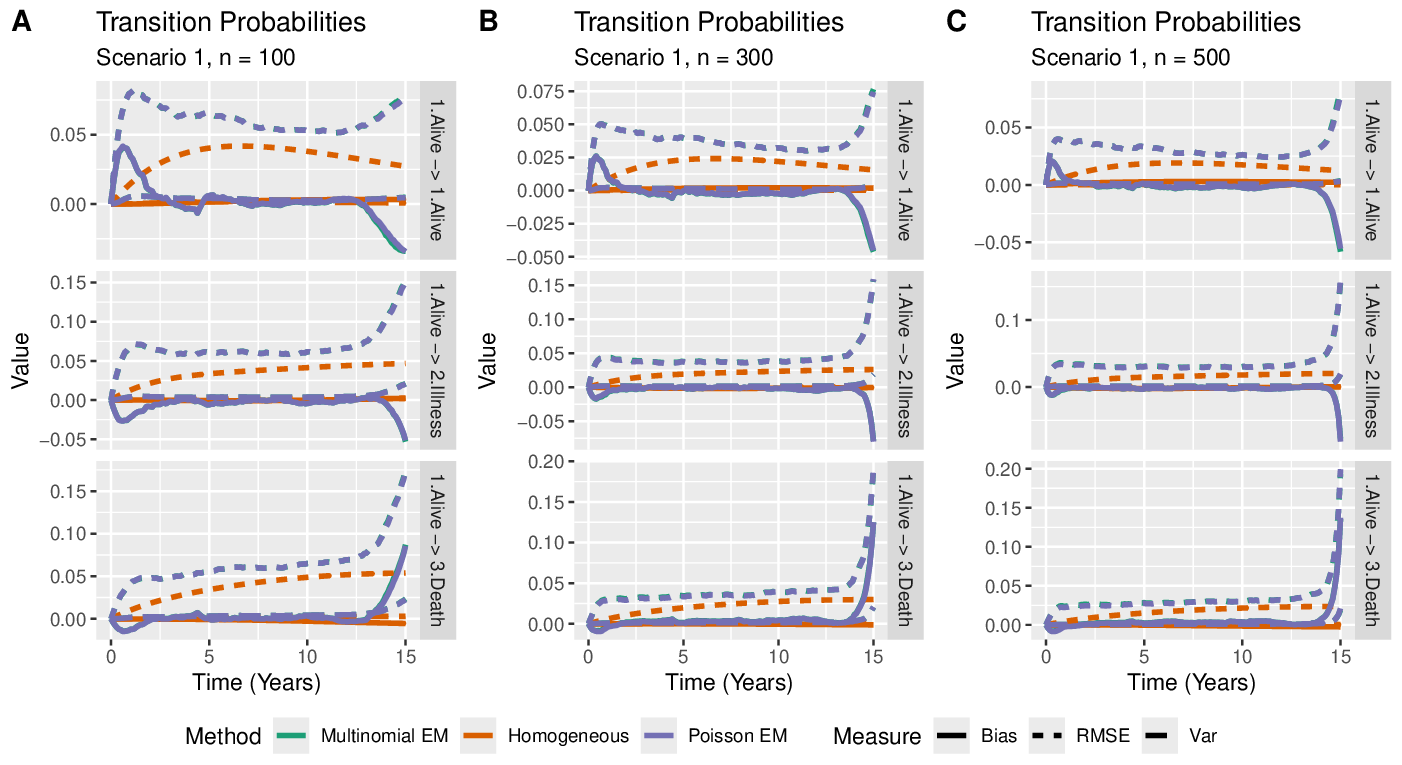}
    \caption{Bias, Variance and RMSE of transition probabilities in scenario 1 for A) $n = 100$, B) $n = 300$, C) $n = 500$ samples in $N = 1000$ simulated data sets.}
    \label{fig:sc1probs}
\end{figure}

\begin{figure}[!ht]
    \centering
    \includegraphics[width = 0.9 \textwidth]{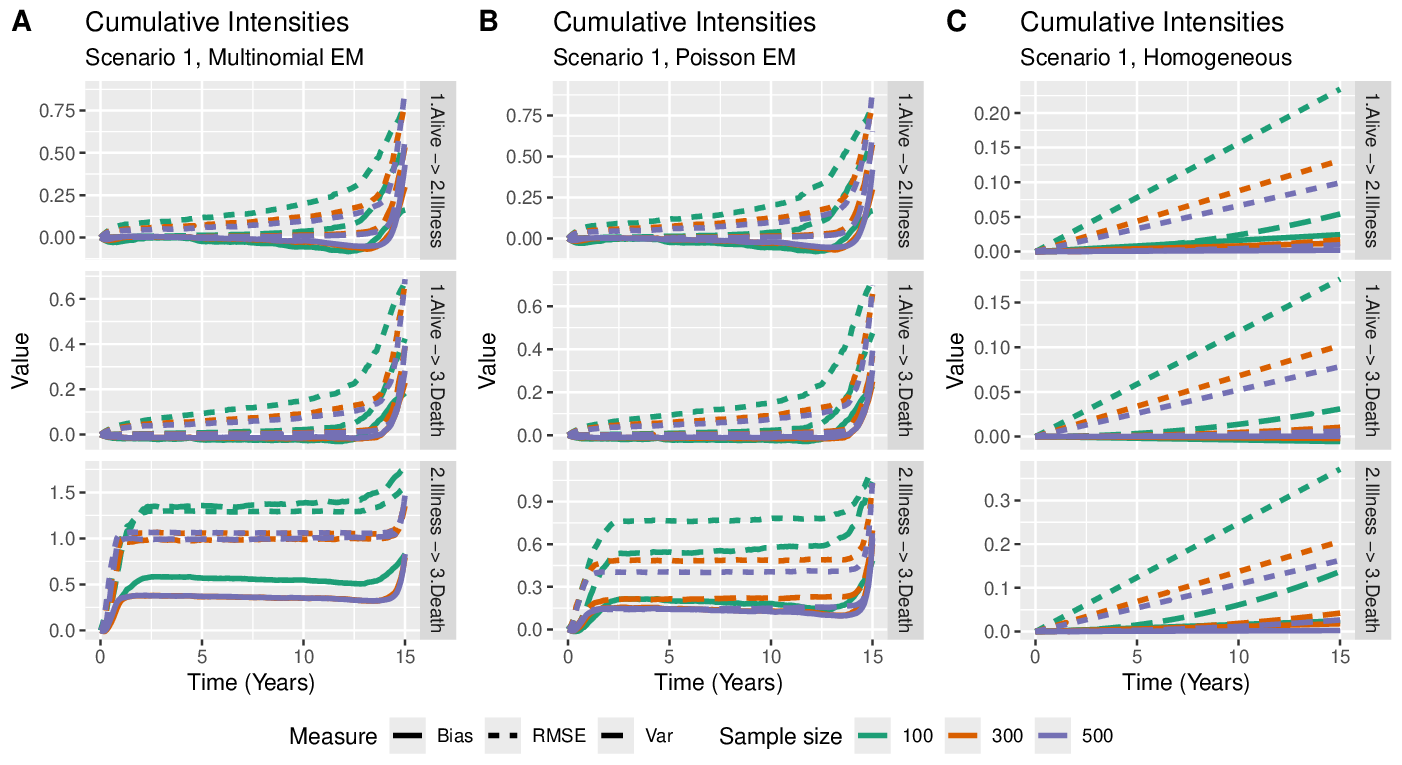}
    \caption{Bias, Variance and RMSE of cumulative intensities in scenario 1 for A) multinomial EM, B) Poisson EM, C) Time-homogeneous methods in $N = 1000$ simulated data sets.}
    \label{fig:sc1compint}
\end{figure}

\begin{figure}[!ht]
    \centering
    \includegraphics[width = 0.9 \textwidth]{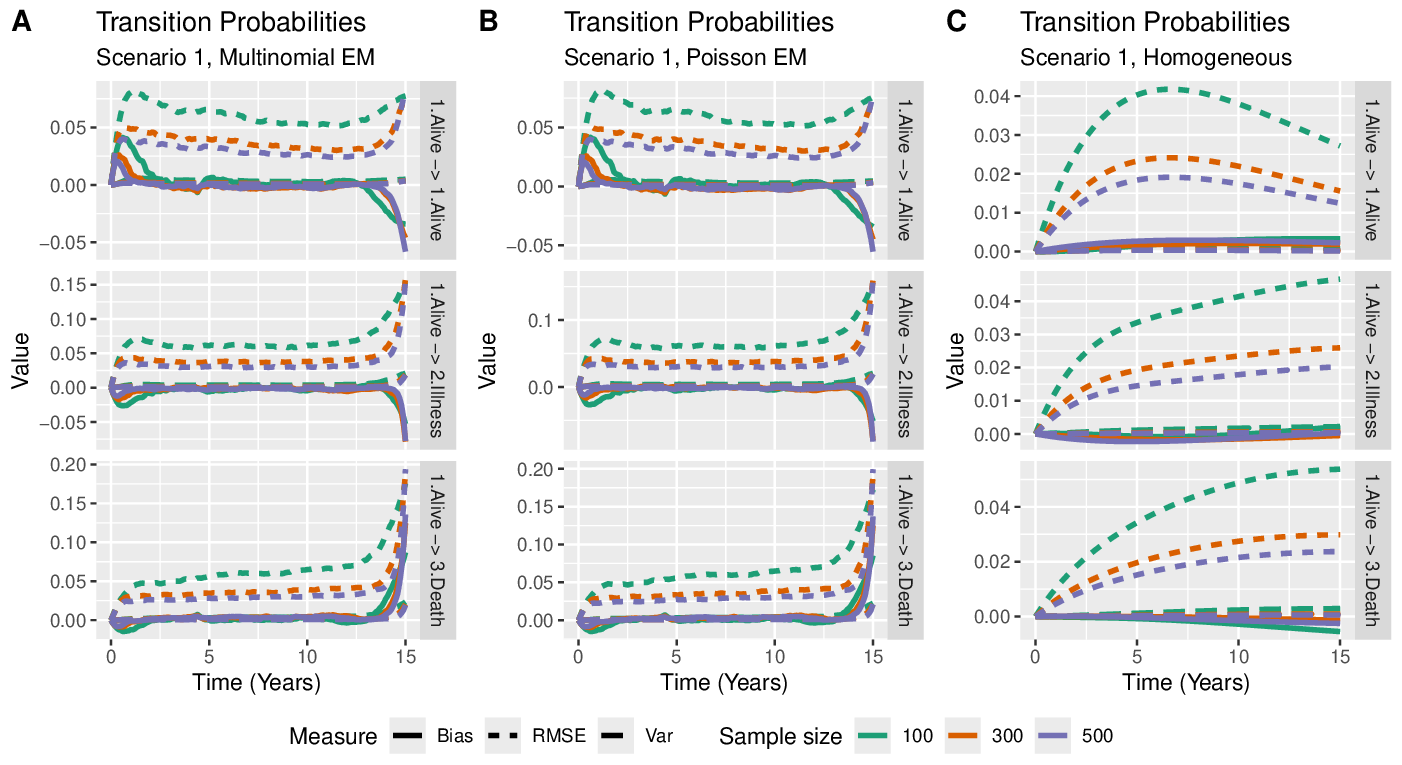}
    \caption{Bias, Variance and RMSE of transition probabilities in scenario 1 for A) multinomial EM, B) Poisson EM, C) Time-homogeneous methods in $N = 1000$ simulated data sets.}
    \label{fig:sc1compprobs}
\end{figure}

\begin{figure}[!ht]
    \centering
    \includegraphics[width = 0.9 \textwidth]{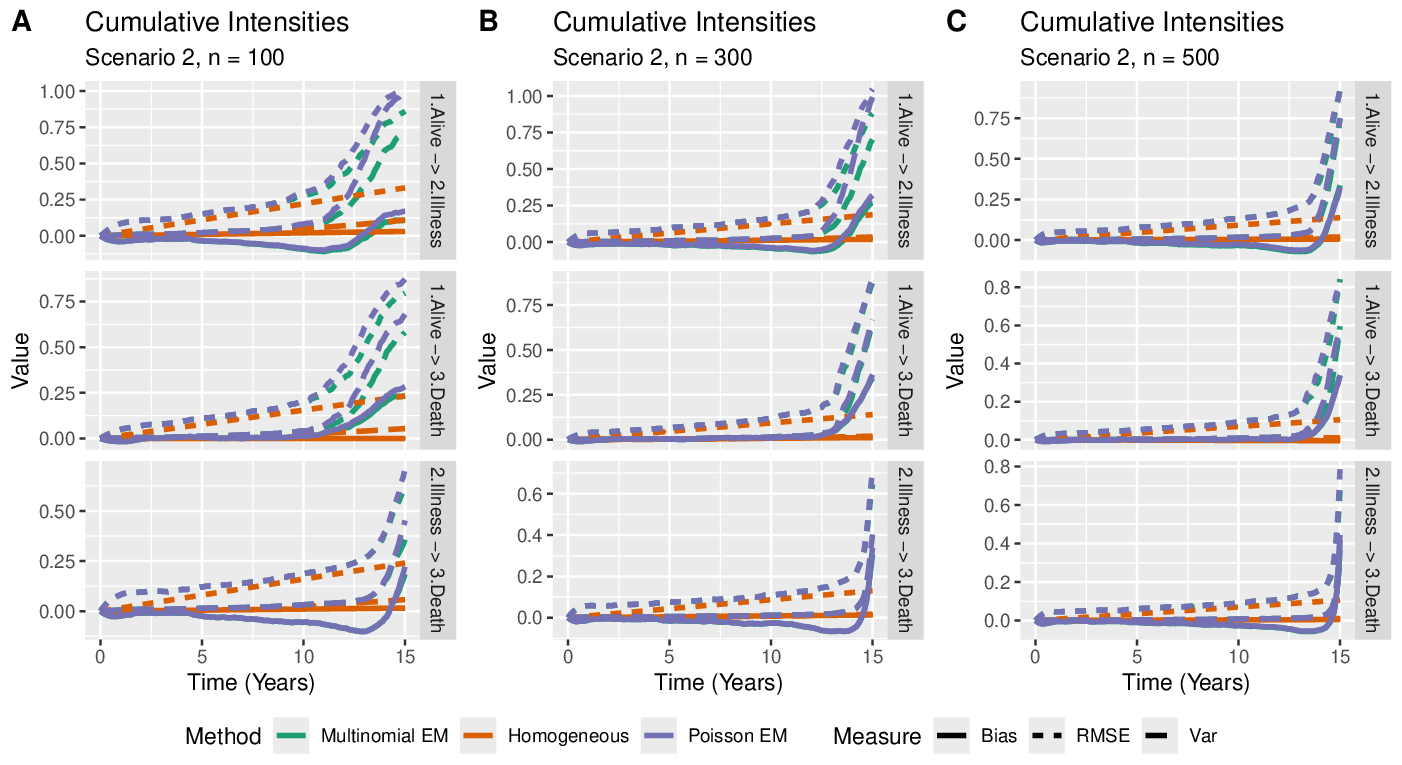}
    \caption{Bias, Variance and RMSE of cumulative intensities in scenario 2 for A) $n = 100$, B) $n = 300$, C) $n = 500$ samples in $N = 1000$ simulated data sets.}
    \label{fig:sc2int}
\end{figure}

\begin{figure}[!ht]
    \centering
    \includegraphics[width = 0.9 \textwidth]{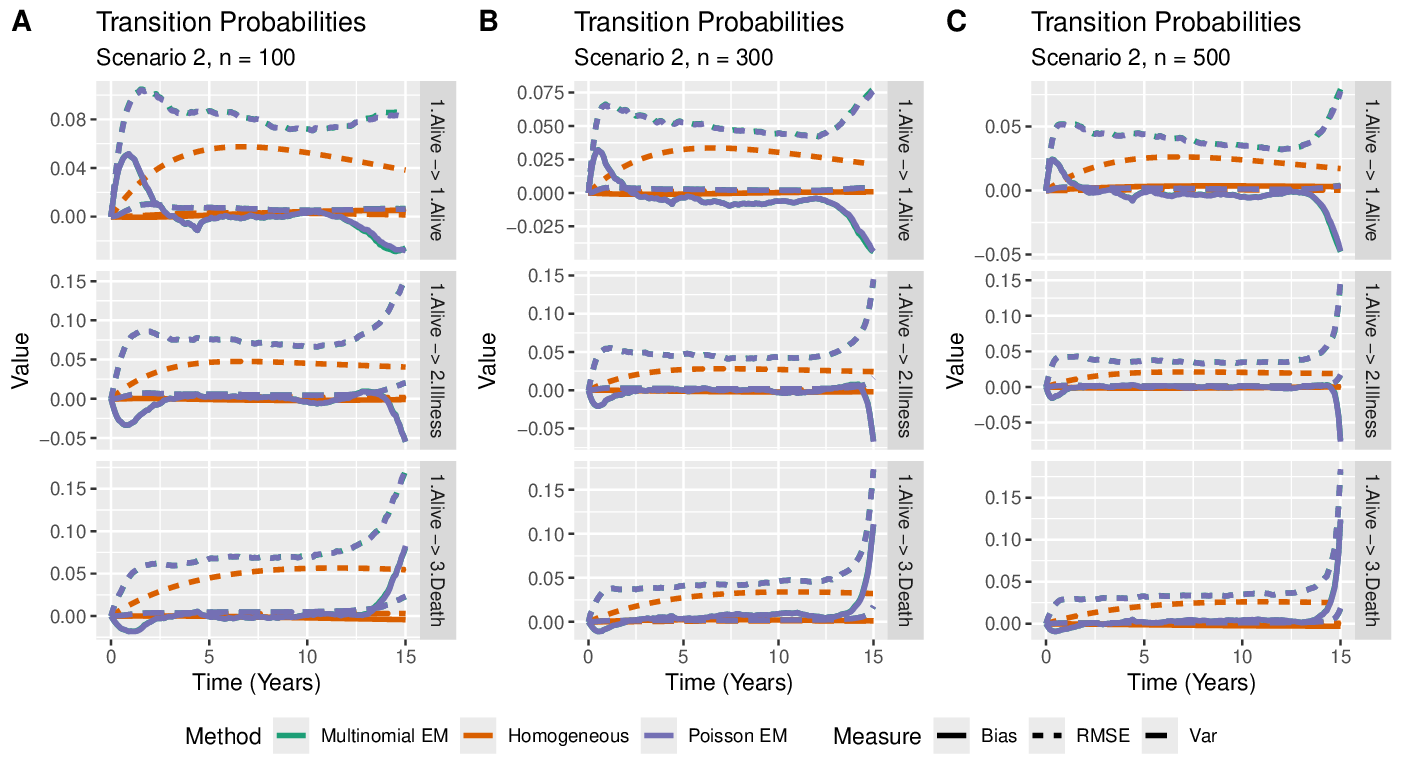}
    \caption{Bias, Variance and RMSE of transition probabilities in scenario 2 for A) $n = 100$, B) $n = 300$, C) $n = 500$ samples in $N = 1000$ simulated data sets.}
    \label{fig:sc2probs}
\end{figure}

\begin{figure}[!ht]
    \centering
    \includegraphics[width = 0.9 \textwidth]{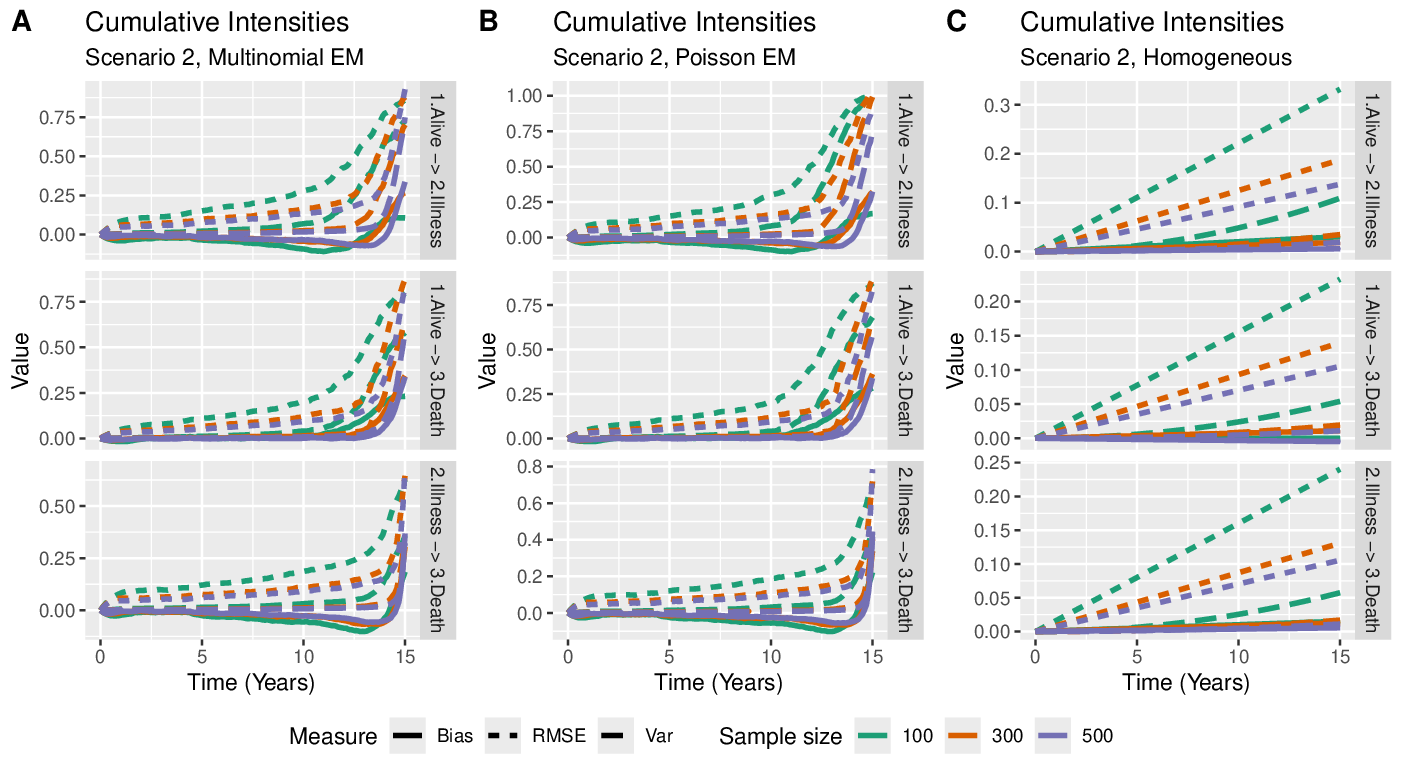}
    \caption{Bias, Variance and RMSE of cumulative intensities in scenario 2 for A) multinomial EM, B) Poisson EM, C) Time-homogeneous methods in $N = 1000$ simulated data sets.}
    \label{fig:sc2compint}
\end{figure}

\begin{figure}[!ht]
    \centering
    \includegraphics[width = 0.9 \textwidth]{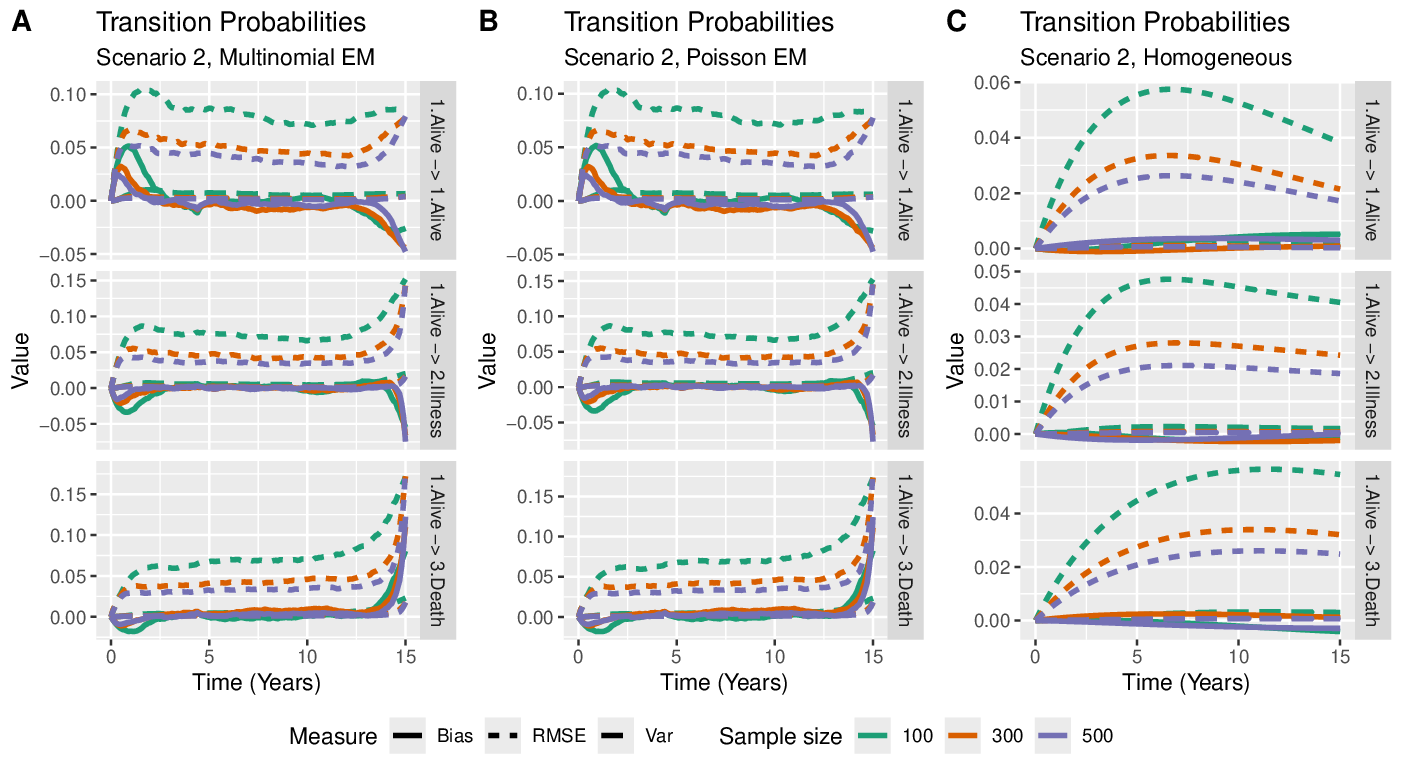}
    \caption{Bias, Variance and RMSE of transition probabilities in scenario 2 for A) multinomial EM, B) Poisson EM, C) Time-homogeneous methods in $N = 1000$ simulated data sets.}
    \label{fig:sc2compprobs}
\end{figure}

\begin{figure}[!ht]
    \centering
    \includegraphics[width = 0.9 \textwidth]{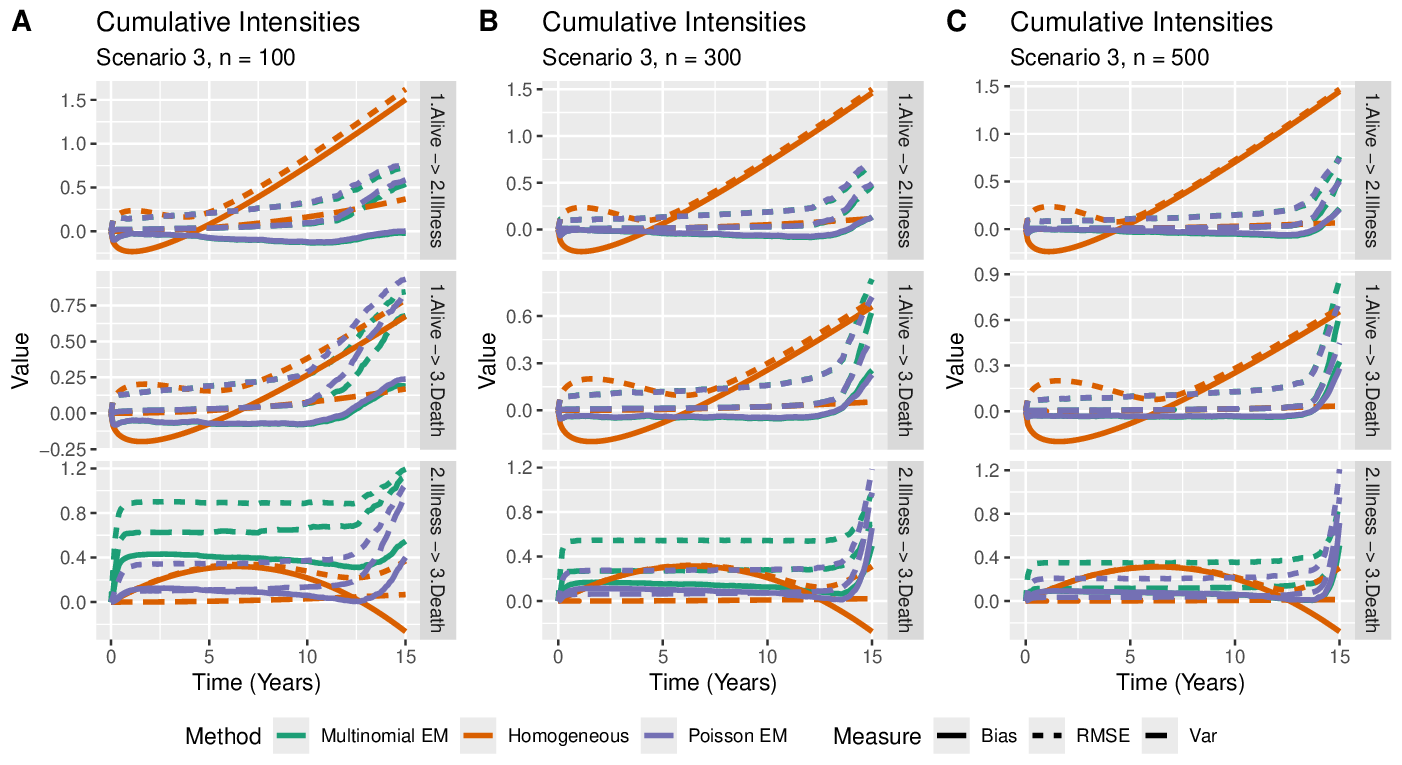}
    \caption{Bias, Variance and RMSE of cumulative intensities in scenario 3 for A) $n = 100$, B) $n = 300$, C) $n = 500$ samples in $N = 1000$ simulated data sets.}
    \label{fig:sc3int}
\end{figure}

\begin{figure}[!ht]
    \centering
    \includegraphics[width = 0.9 \textwidth]{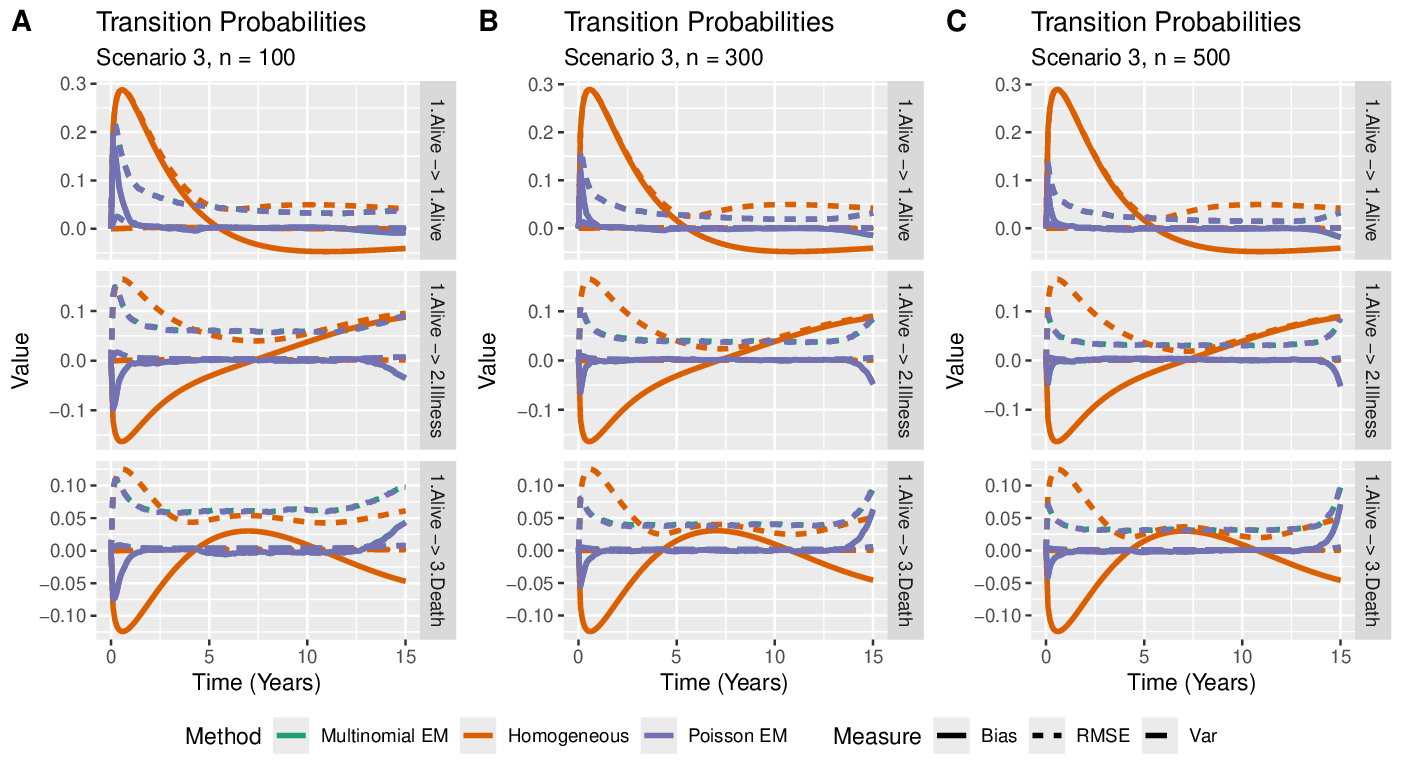}
    \caption{Bias, Variance and RMSE of transition probabilities in scenario 3 for A) $n = 100$, B) $n = 300$, C) $n = 500$ samples in $N = 1000$ simulated data sets.}
    \label{fig:sc3probs}
\end{figure}

\begin{figure}[!ht]
    \centering
    \includegraphics[width = 0.9 \textwidth]{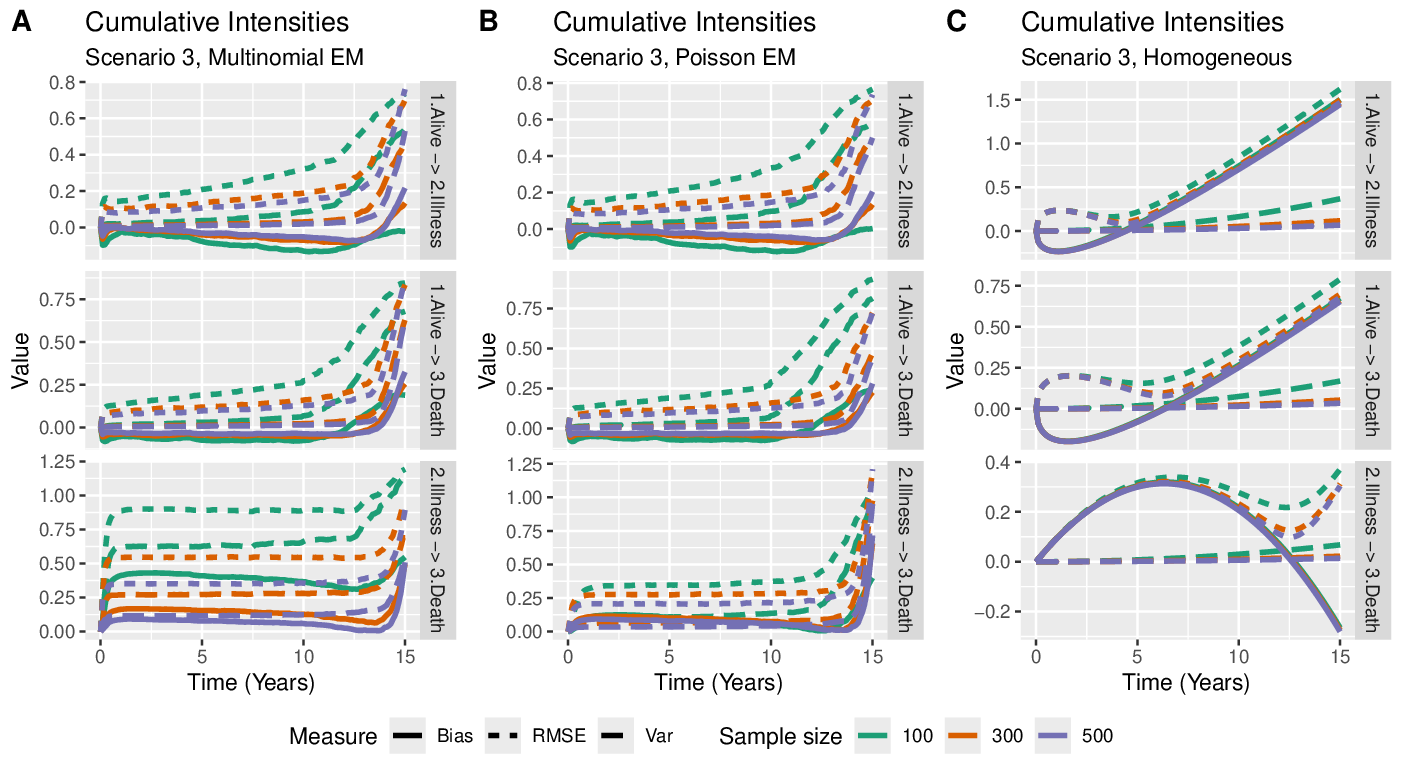}
    \caption{Bias, Variance and RMSE of cumulative intensities in scenario 3 for A) multinomial EM, B) Poisson EM, C) Time-homogeneous methods in $N = 1000$ simulated data sets.}
    \label{fig:sc3compint}
\end{figure}

\begin{figure}[!ht]
    \centering
    \includegraphics[width = 0.9 \textwidth]{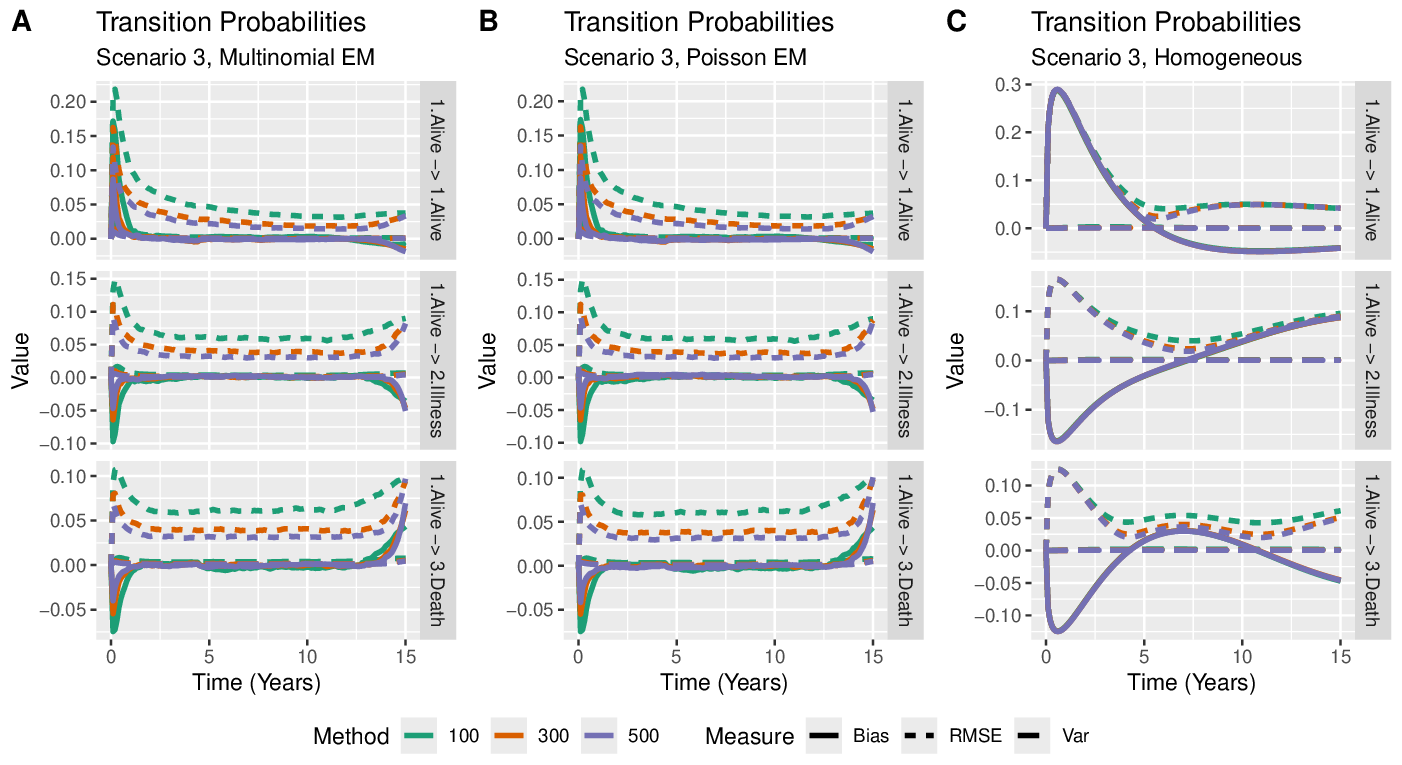}
    \caption{Bias, Variance and RMSE of transition probabilities in scenario 3 for A) multinomial EM, B) Poisson EM, C) Time-homogeneous methods in $N = 1000$ simulated data sets.}
    \label{fig:sc3compprobs}
\end{figure}

\begin{figure}[!ht]
    \centering
    \includegraphics[width = 0.9 \textwidth]{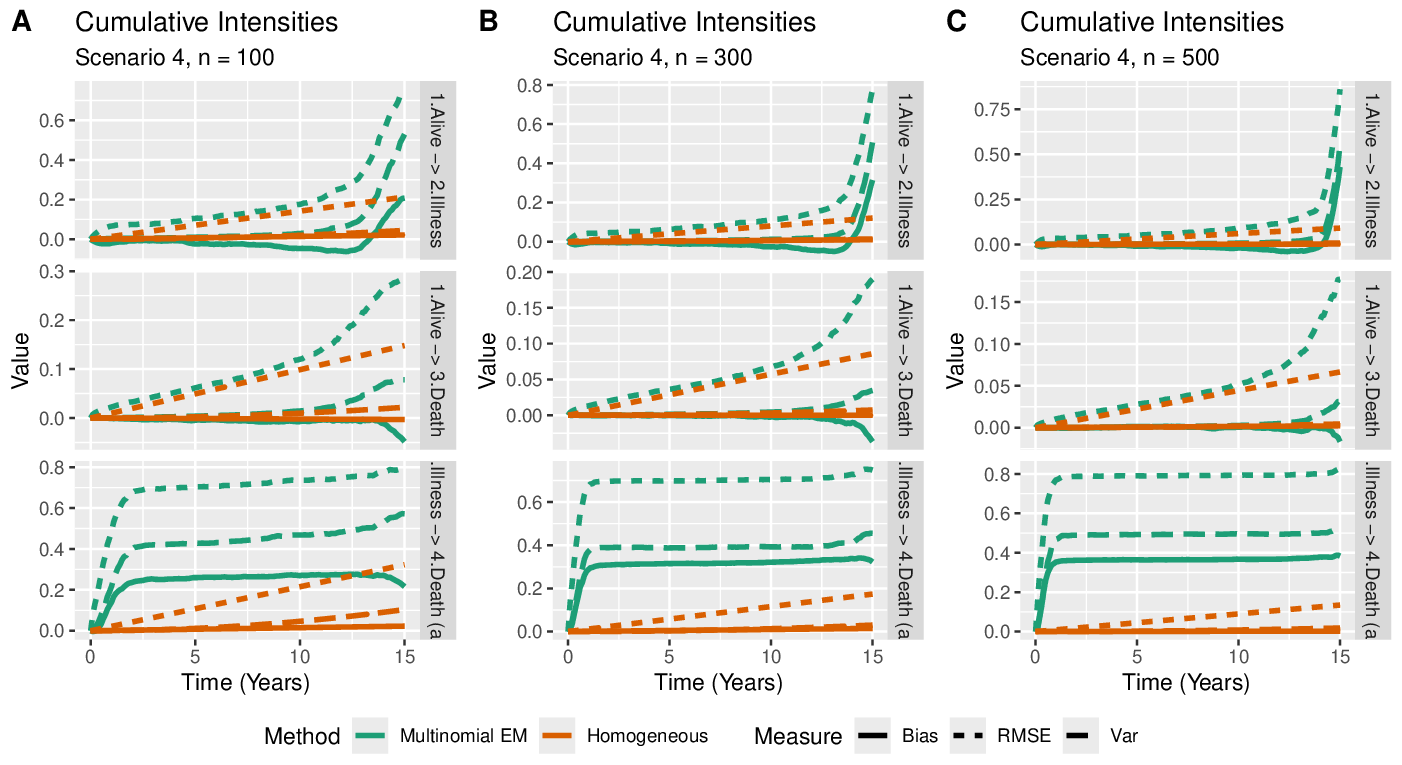}
    \caption{Bias, Variance and RMSE of cumulative intensities in scenario 4 for A) $n = 100$, B) $n = 300$, C) $n = 500$ samples in $N = 1000$ simulated data sets.}
    \label{fig:sc4int}
\end{figure}

\begin{figure}[!ht]
    \centering
    \includegraphics[width = 0.9 \textwidth]{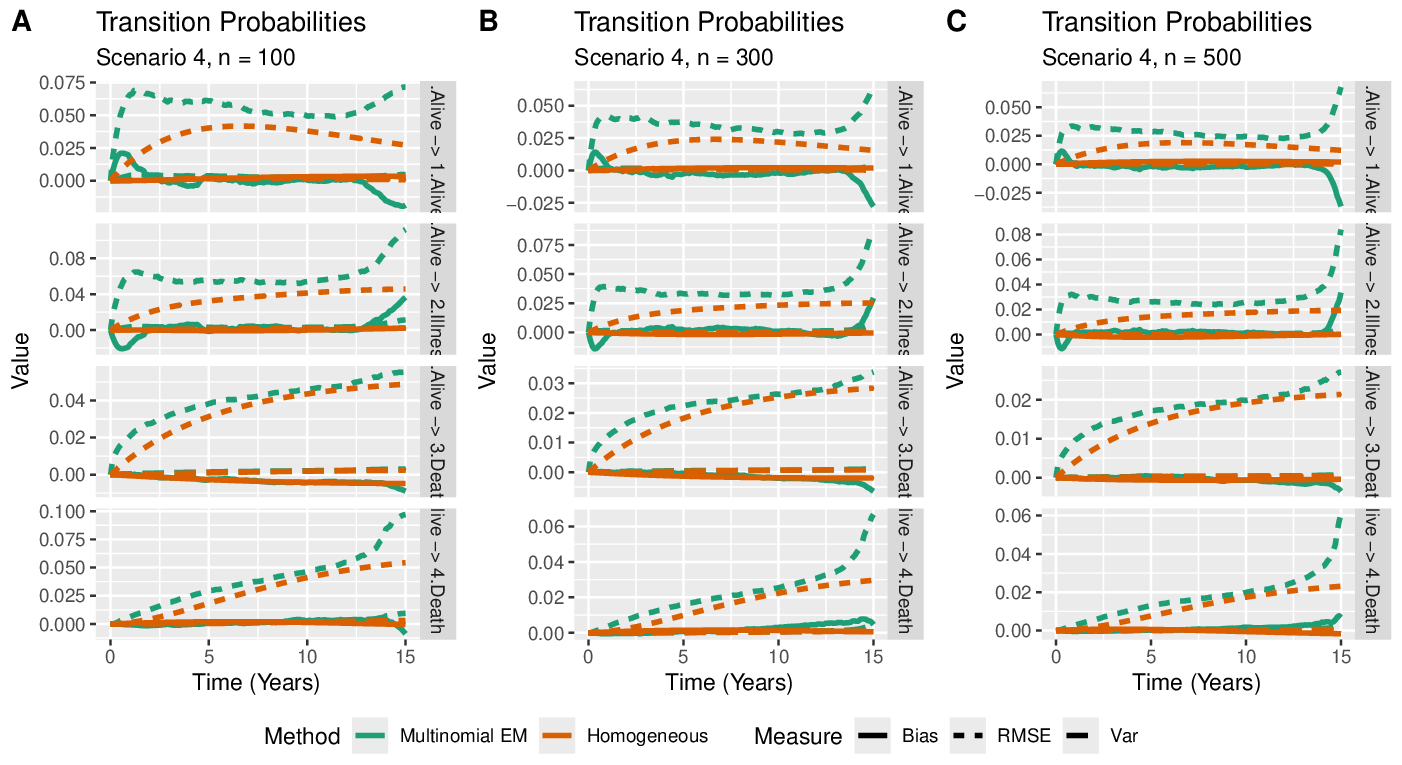}
    \caption{Bias, Variance and RMSE of transition probabilities in scenario 4 for A) $n = 100$, B) $n = 300$, C) $n = 500$ samples in $N = 1000$ simulated data sets.}
    \label{fig:sc4probs}
\end{figure}

\begin{figure}[!ht]
    \centering
    \includegraphics[width = 0.9 \textwidth]{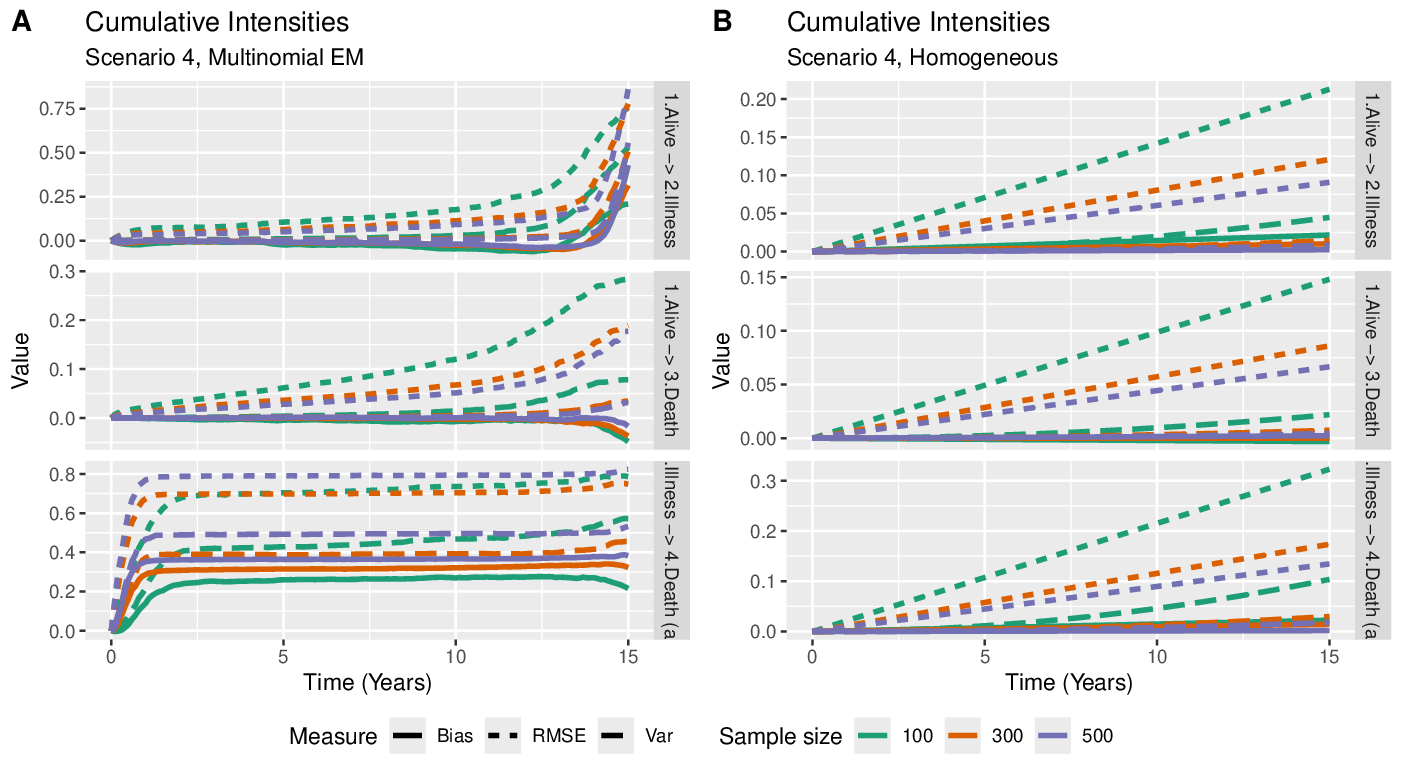}
    \caption{Bias, Variance and RMSE of cumulative intensities in scenario 4 for A) multinomial EM, B) Time-homogeneous methods in $N = 1000$ simulated data sets.}
    \label{fig:sc4compint}
\end{figure}

\begin{figure}[!ht]
    \centering
    \includegraphics[width = 0.9 \textwidth]{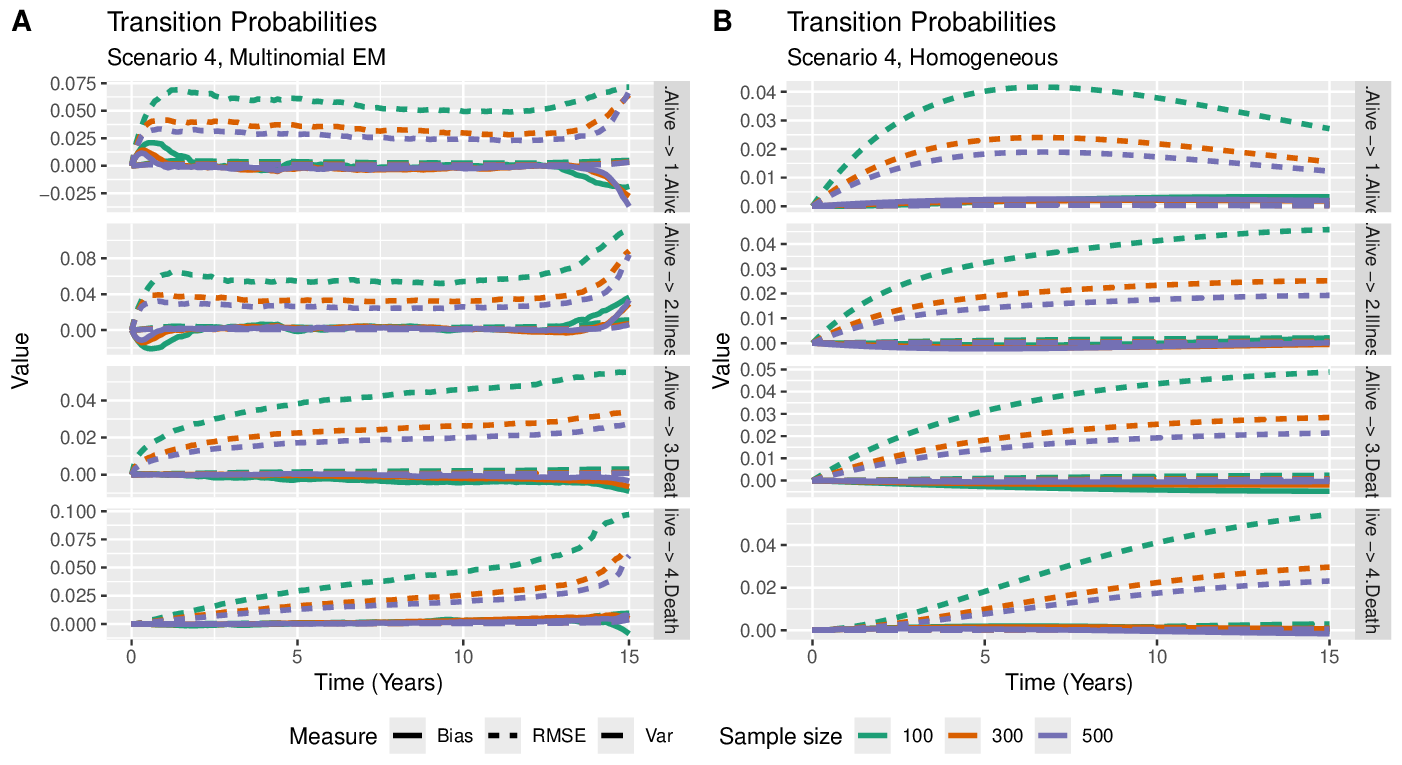}
    \caption{Bias, Variance and RMSE of transition probabilities in scenario 4 for A) multinomial EM, B) Poisson EM methods in $N = 1000$ simulated data sets.}
    \label{fig:sc4compprobs}
\end{figure}

\begin{figure}[!ht]
    \centering
    \includegraphics[width = 0.9 \textwidth]{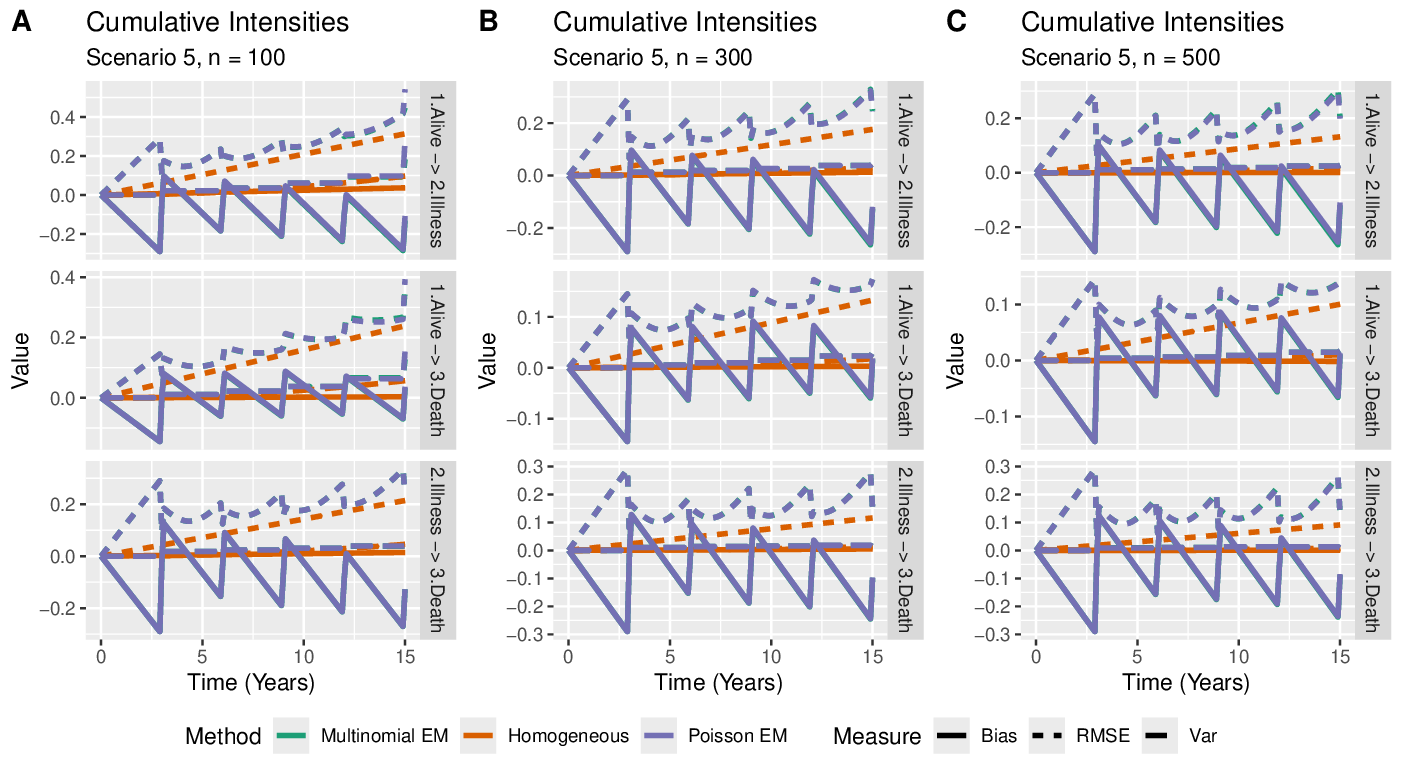}
    \caption{Bias, Variance and RMSE of cumulative intensities in scenario 5 for A) $n=100$ B) $n=300$ C) $n = 500$ samples in $N = 1000$ simulated data sets.}
    \label{fig:sc5compint}
\end{figure}

\begin{figure}[!ht]
    \centering
    \includegraphics[width = 0.9 \textwidth]{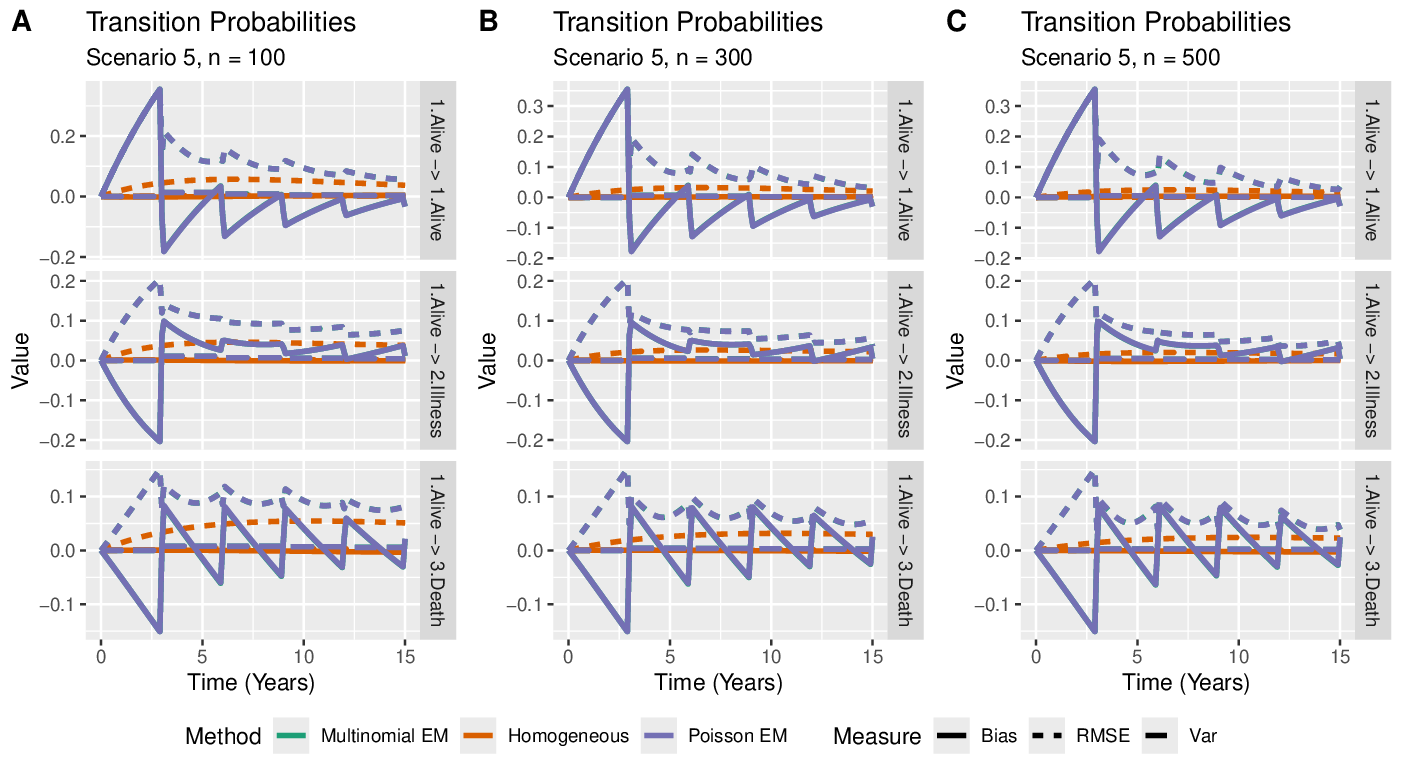}
    \caption{Bias, Variance and RMSE of transition probabilities in scenario 5 for A) $n=100$ B) $n=300$ C) $n = 500$ samples in $N = 1000$ simulated data sets.}
    \label{fig:sc5compprobs}
\end{figure}

\begin{figure}[!ht]
    \centering
    \includegraphics[width = 0.9 \textwidth]{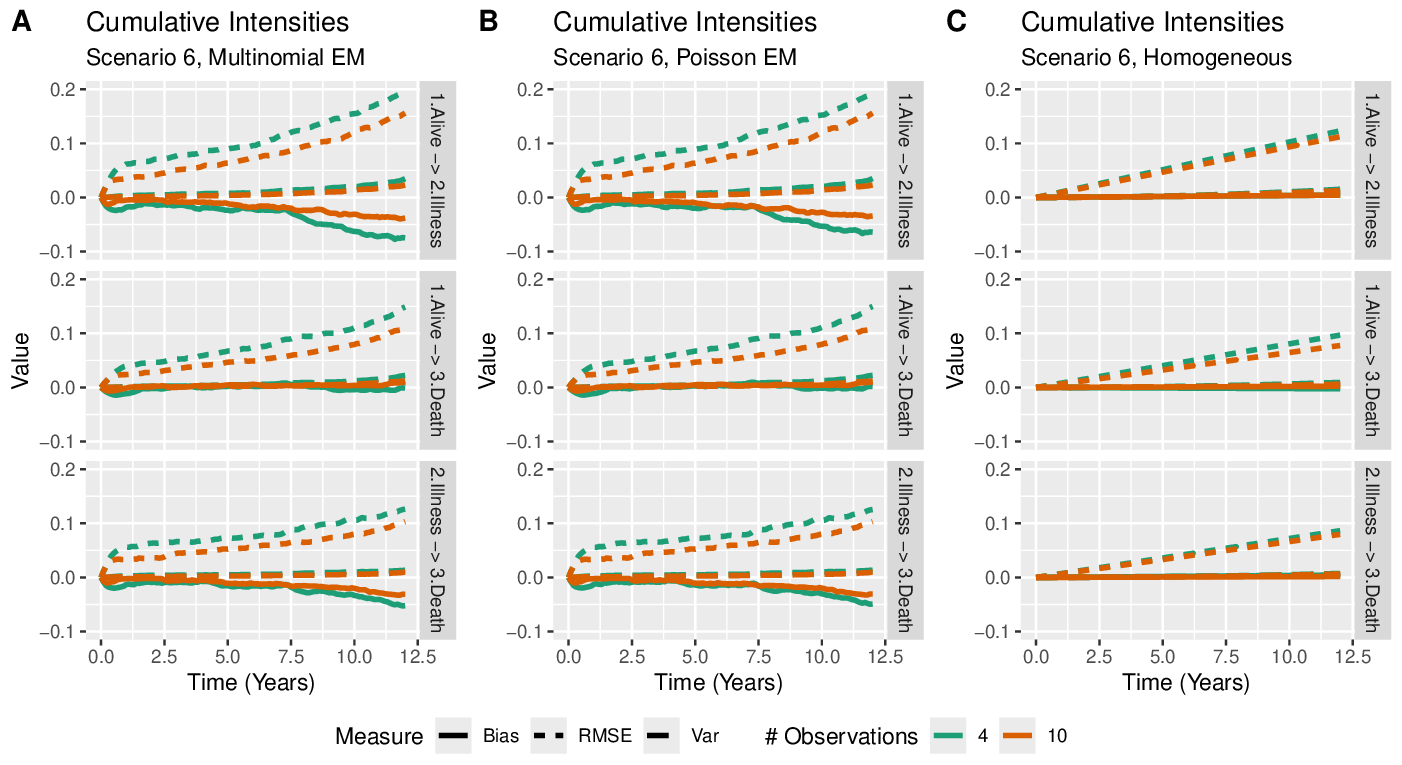}
    \caption{Bias, Variance and RMSE of cumulative intensities in scenario 6 for A) multinomial EM B) Poisson EM C) Time-homogeneous methods in $N = 1000$ simulated data sets for different numbers of observation times.}
    \label{fig:sc6compint}
\end{figure}

\begin{figure}[!ht]
    \centering
    \includegraphics[width = 0.9 \textwidth]{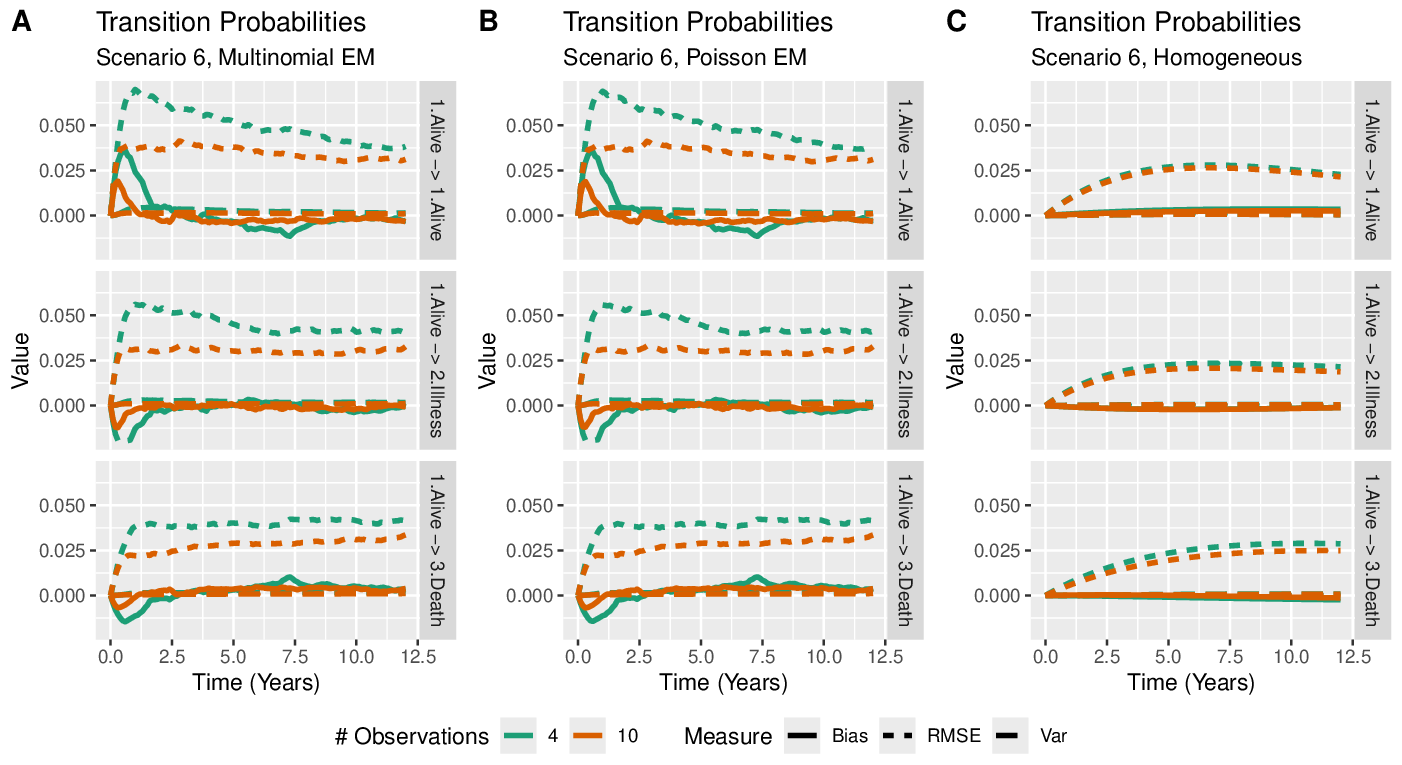}
    \caption{Bias, Variance and RMSE of transition probabilities in scenario 6 for A) multinomial EM B) Poisson EM C) Time-homogeneous methods in $N = 1000$ simulated data sets for different numbers of observation times.}
    \label{fig:sc6compprobs}
\end{figure}

\end{document}
